# Supplementary material for: Investigating the Electronic and Magnetic Properties of Na$_x$Fe$_{1/2}$Mn$_{1/2}$O$_2$ Cathode Materials with X-ray Compton Scattering
Source: arXiv:2602.12378 ancillary file (2026-02-12)
Supplement: Supplementary file 1 [file SM.pdf]

# Supplemental material: Investigating the Electronic and Magnetic Properties of $Na_xFe_{1/2}Mn_{1/2}O_2$ Cathode Materials with x-ray Compton Scattering

Veenavee Nipunika Kothalawala[a,*], Kosuke Suzuki[b], Johannes Nokelainen[a,c,d,e], Ilja Makkonen[f], Erica West[g], Lassi Roininen[g], Jere Leinonen[h,i], Pekka Tynjälä[h,i], Petteri Laine[h,i], Juho Välikangas[h,i], Ulla Lassi[h,i], Assa Aravindh Sasikala Devi[h,j,*], Matti Alatalo[k], Yuki Mizuno[l], Naruki Tsuji[l], Hikaru Usami[b], Yuju Nagasaki[b], Tsuyoshi Takami[m], Yoshiharu Sakurai[l], Hiroshi Sakurai[b], Mohammad Babar[n], Venkat Vishwanathan[n], Arun Bansil[d,e], and Bernardo Barbiellini[a,d,e]

[a]*Department of Physics, School of Engineering Sciences, LUT University, FI-53851 Lappeenranta, Finland*
[b]*Graduate School of Science and Technology, Gunma University, Kiryu, Gunma 376-8515, Japan*
[c]*Department of Mechanical Engineering, School of Energy Systems, LUT University, FI-53851 Lappeenranta, Finland*
[d]*Department of Physics, Northeastern University, Boston, Massachusetts 02115, USA*
[e]*Quantum Materials and Sensing Institute, Northeastern University, Burlington, MA 01803, USA*
[f]*Department of Physics, University of Helsinki, P.O. Box 43, FI-00014 University of Helsinki, Helsinki, Finland*
[g]*Department of Physics, Northeastern University, Boston, Massachusetts 02115, USA*
[h]*Research Unit of Sustainable Chemistry, University of Oulu, Oulu, Finland*
[i]*Kokkola University Consortium Chydenius, University of Jyväskylä, Kokkola, Finland*
[j]*Materials and Mechanical Engineering Research Unit,University of Oulu, Oulu, Finland*
[k]*Nano and Molecular Systems Research Unit, University of Oulu, Pentti Kaiteran Katu 1, 90570 Oulu, Finland*
[l]*Japan Synchrotron Radiation Research Institute (JASRI), Sayo, Hyogo 679-5198, Japan*
[m]*Otemon Gakuin University, 2-1-15 Nishiai, Ibaraki, Osaka 567-8502, Japan*
[n]*College of Engineering, Aerospace Engineering, University of Michigan, Ann Arbor, MI 48109 USA*
[*]Veenavee.kothalawala@lut.fi, Assa.Sasikaladevi@oulu.fi

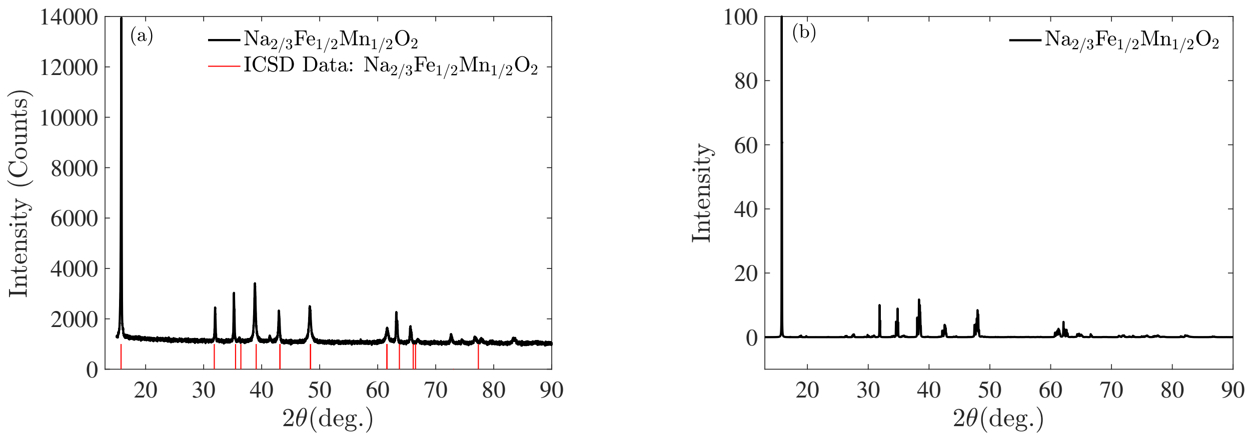


Figure S1: x-ray diffraction (XRD) patterns at the $CuK_\alpha$ fluorescence of $Na_{2/3}Fe_{1/2}Mn_{1/2}O_2$. (a) Experimental data. (b) Calculated pattern generated using VESTA software on the P2 phase model.

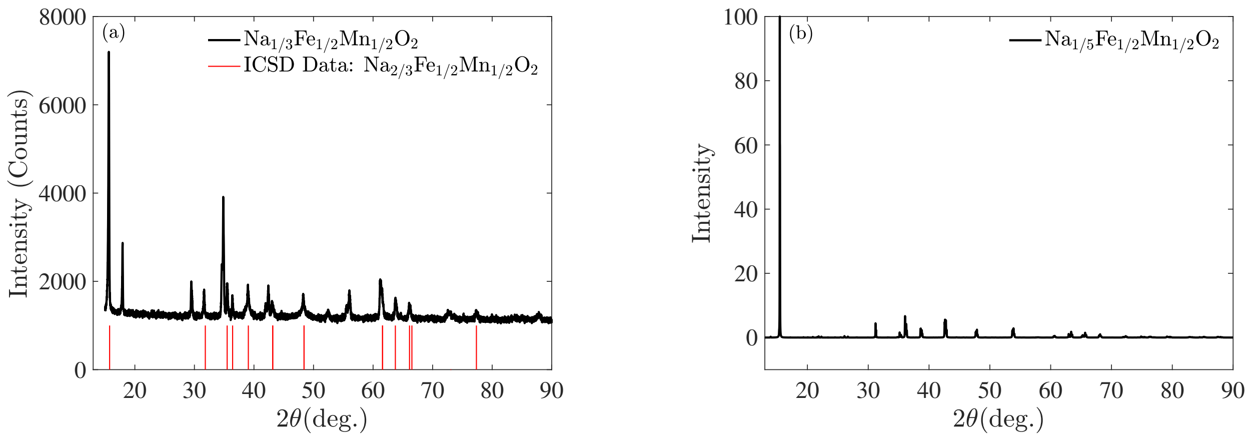


Figure S2: XRD patterns at the $CuK_\alpha$ fluorescence of $Na_{1/3}Fe_{1/2}Mn_{1/2}O_2$. (a) Experimental data showing a P2 phase contaminated by a secondary phase, which likely originates from incomplete formation of the layered structure under sodium-deficient conditions, leaving residual Na-poor oxides or related intermediate phases. (b) Calculated pattern generated using VESTA software on the O2 phase model for $Na_{1/5}Fe_{1/2}Mn_{1/2}O_2$.

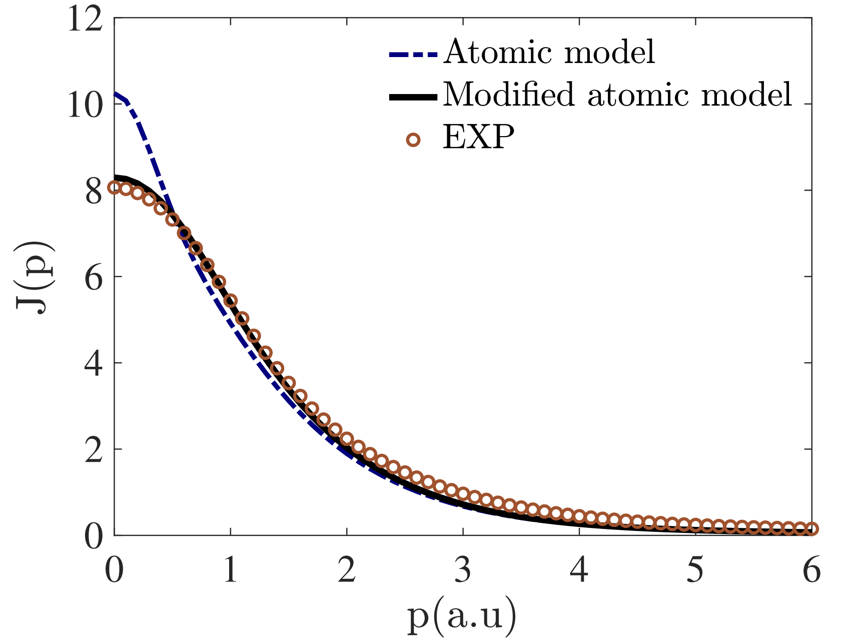


Figure S3: Spherically-averaged theoretical and experimental valence Compton profiles of $Na_{1/3}Fe_{1/2}Mn_{1/2}O_2$. Theoretical profiles are convoluted with a Gaussian of 0.5 a.u. full-width-at-half-maximum.

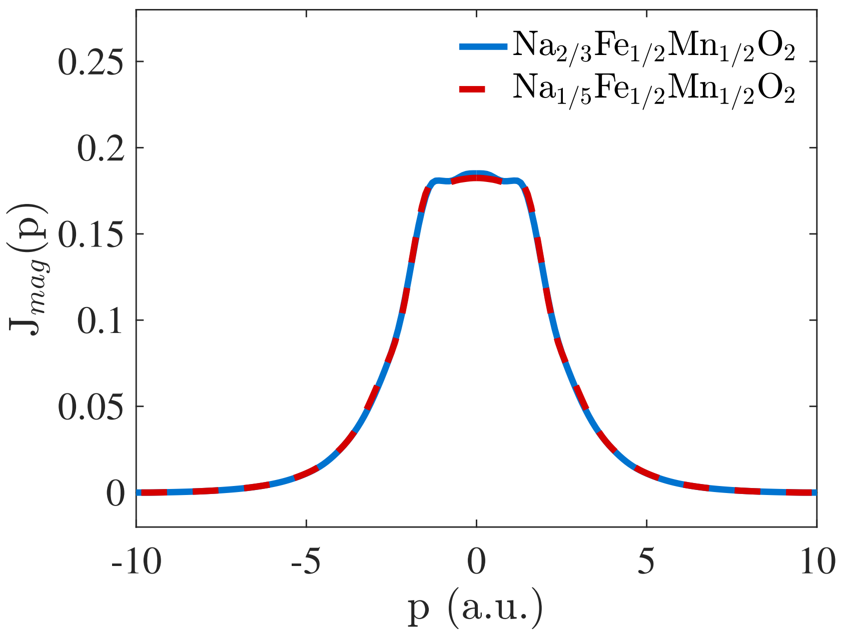


Figure S4: Spherically-averaged DFT based magnetic Compton profiles for $Na_{2/3}Fe_{1/2}Mn_{1/2}O_2$, and $Na_{2/9}Fe_{1/2}Mn_{1/2}O_2$. Two profiles are remarkably similar in that they can be collapsed onto a single curve when normalized to the same (unit) area.

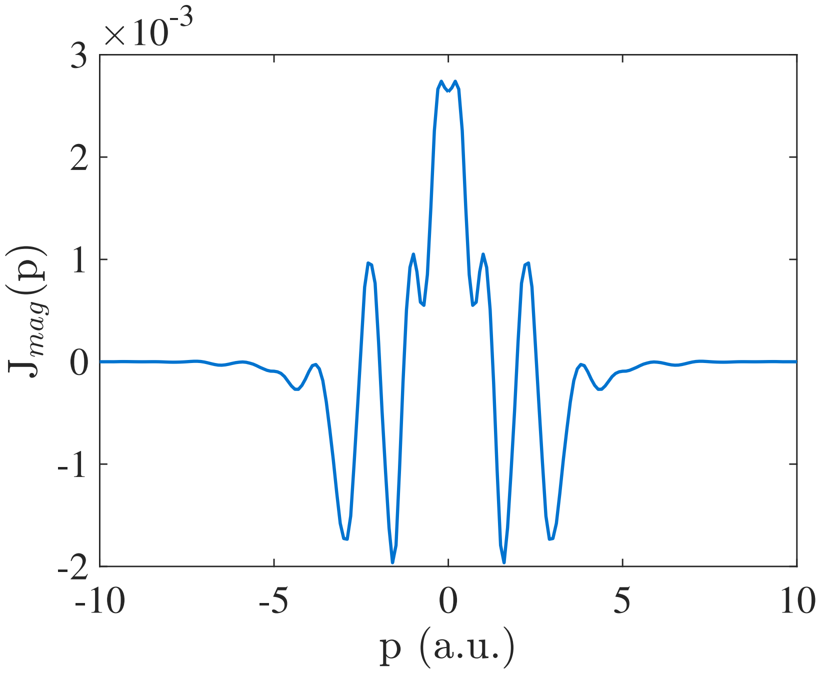


Figure S5: Difference between the spherically-averaged magnetic Compton profile of $Na_{2/3}Fe_{1/2}Mn_{1/2}O_2$ minus the same profile for $Na_{2/9}Fe_{1/2}Mn_{1/2}O_2$ based on DFT computations, where both profiles are normalized to the same (unit) area.

# S1 Supplemental Data

All the data from the r2SCAN are provided at the Github repository: https://github.com/Veenavi92/NFMO_r2SCAN
